# Supplementary material for: Characterization of Optical and Spin Properties of Single Tin-Vacancy Centers in Diamond Nanopillars
Source: arXiv:1811.09941 source file (2019-04-29)
Supplement: Supplementary file 1 [file supplement.pdf]

# Supplemental Materials for Optical Characterization of Single Tin-Vacancy Centers in Diamond Nanopillars

Alison E. Rugar, Constantin Dory, Shuo Sun, and Jelena Vučković

*E. L. Ginzton Laboratory, Stanford University, Stanford, CA 94305, USA*

## I. SETUPS

To acquire the data presented in the main text, we use two different setups. The photoluminescence measurements at at zero magnetic field, including $g^{(2)}[\tau]$ and polarization dependence measurements, are performed in a home-built scanning confocal microscope, shown schematically in Fig. S1. We use a 532-nm laser to excite the emitter and collect the signal into an optical fiber. To spectrally filter for the zero-phonon lines, we have a 568-nm long-pass (568LP), a 594LP, a 532-nm notch (532N), and a 700-nm short-pass (700SP) filter on the collection for most optical measurements. The sample is held at 5 K in a Montana Instruments Cryostation. The polarization optics in Fig. S1 were removed for $g^{(2)}[\tau]$ and other photoluminescence measurements in which polarization was not studied.

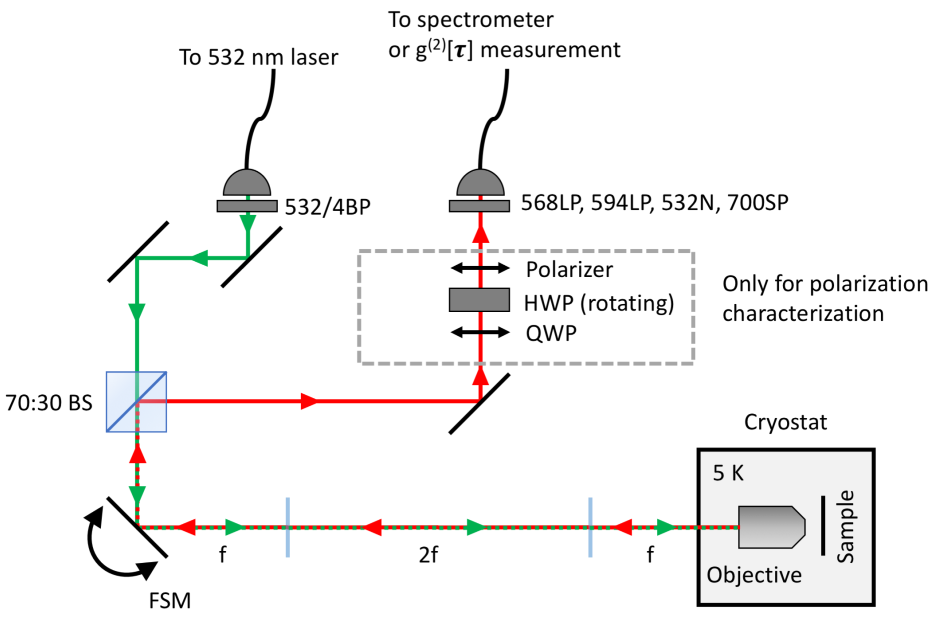


FIG. S1. Schematic drawing of optical path during photoluminescence, polarization, and $g^{(2)}[\tau]$ measurements. Green indicates excitation path (532 nm). Red indicates detection path ($\sim$ 620 nm). The optical components are beam splitter (BS) reflectance:transmittance (R:T), mirror (black diagonal lines), lenses (vertical blue lines) focal length $f$, fast steering mirror (FSM), quarter-wave plate (QWP), and half-wave plate (HWP).

Measurements in a magnetic field are performed with the second setup, shown in Fig. S2. This setup incorporates an attoDRY2100 cryostat with a superconducting magnet. The configuration for photoluminescence studies with 532-nm excitation is shown in Fig. S2. For

photoluminescence excitation, we use a 620/14 band-pass filter on the resonant excitation, a 532/25 on the 532-nm repump, and 638LP and 661/20 filters on the detection before a multimode fiber. The 532/4 filter is removed from the excitation path shown in Fig. S2. The flip mirror of Fig. S2 is used to direct the emission to a multimode fiber that goes to a single photon counting module. The scanning resonant laser we use is the MSquared SolsTiS with an External Mixing Module.

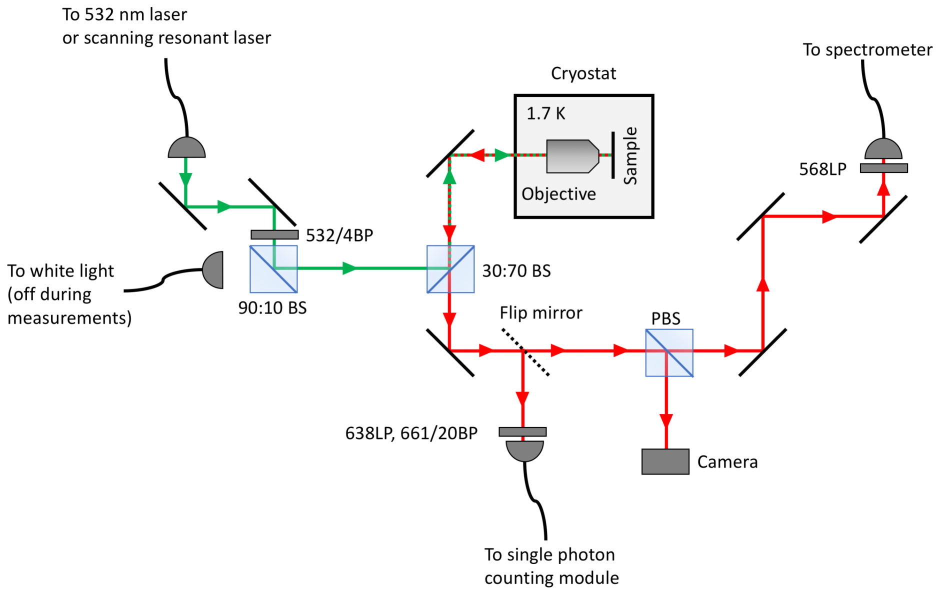


FIG. S2. Schematic drawing of optical path during magnetic field measurements. Green indicates excitation path (532 nm). Red indicates detection path ($\sim 620$ nm). Optical components labeled as before in Fig. S1, with the additions: polarizing beam splitter (PBS) and flip mirror.

## II. BROAD PHOTOLUMINESCENCE SPECTRUM

To get the background-subtracted data shown in Fig. 3 of the main text, we acquired the spectrum from a pillar that did not contain a $SnV^-$ and subtracted it from the raw data. Plots of both the background spectrum and the raw spectrum from the pillar of interest can be found in Fig. S3.

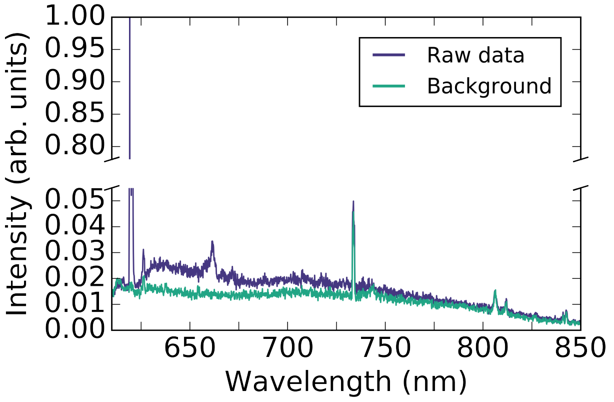


FIG. S3. Photoluminescence spectra of the raw data from a pillar containing a $SnV^-$ center and the background spectrum collected from a pillar without a $SnV^-$ under the same conditions of excitation power and integration time.

## III. SPECTRA FOR DIFFERENT $B_{z'}$

In this section we present the spectra from which we find the outer peaks locations that are presented in Figs. 5(c) and (e) in the main text. These data are collected at 1.7 K via photoluminescence spectroscopy with a single monochromator. The excitation laser is of wavelength 532 nm and power $\sim$ 1 mW. A 568LP filter is used in the collection path. A half-wave plate was placed in front of the PBS in the collection path when needed to increase the signal transmitted through the PBS to the detection fiber. The Lorentzian fits were found with the SciPy function `curve_fit` in Python.

To extract the data shown in Figs. 5(c) and (e) in the main text for the two spin-conserving transitions, we fit the double monochromator data to double Lorentzians. Likewise, we fit the single monochromator data to quadruple Lorentzians to extract the outer, spin non-conserving transition frequencies. These fits are shown as solid red curves in Figs. S4 and S5. We omit the data points in Figs. 5(c) and (e) of the main text where a good fit was not achieved.

## IV. SATURATION

We attempted to saturate our $SnV^-$. However, with the 532-nm power that we had available, we did not leave the linear regime, as shown in Fig. S6. This result is consistent

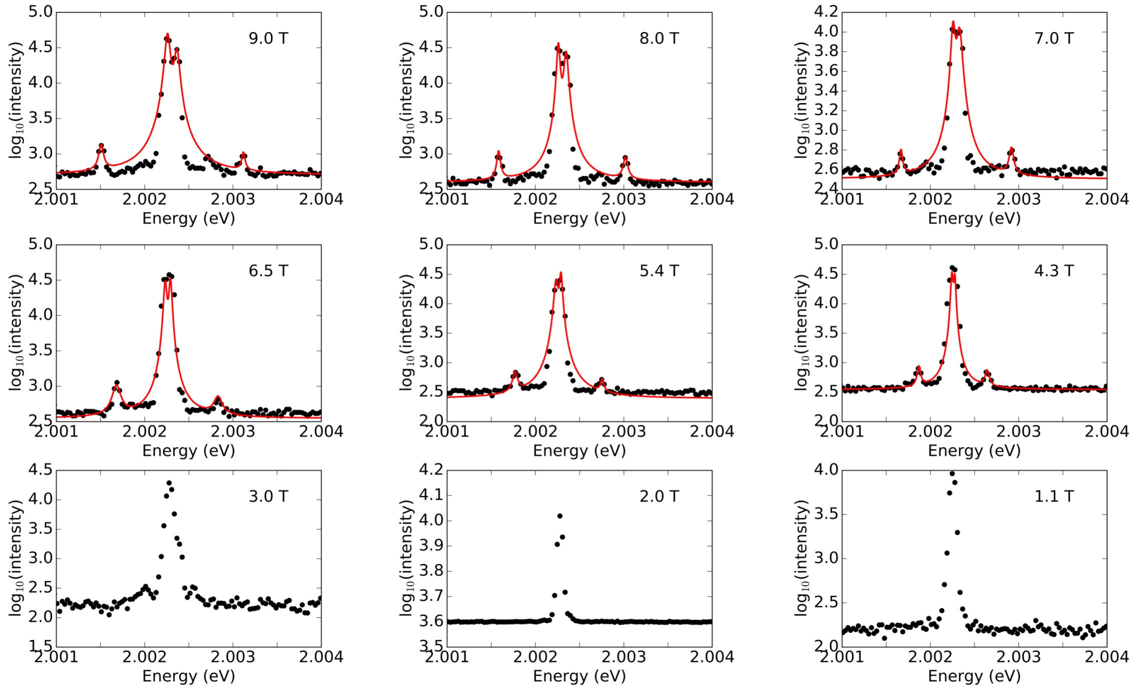


FIG. S4. Single monochromator spectra of C transitions at different magnetic fields at 1.7 K. Field at which data are acquired is indicated in the upper-right corner of each plot. Intensity (y-axis) on a $\log_{10}$ scale. Solid red lines are Lorentzian fits to the data. Unfitted spectra correspond to the omitted data points in the main text Fig. 5(c).

with the saturation behavior reported by Iwasaki *et al.* [1]. We measured the emission into the C and D zero-phonon lines by fitting Lorentzians to the spectra acquired at each power measured at the objective and computing the area underneath the Lorentzians.

---

[1] T. Iwasaki, Y. Miyamoto, T. Taniguchi, P. Siyushev, M. H. Metsch, F. Jelezko, and M. Hatano, Phys. Rev. Lett. **119**, 253601 (2017).

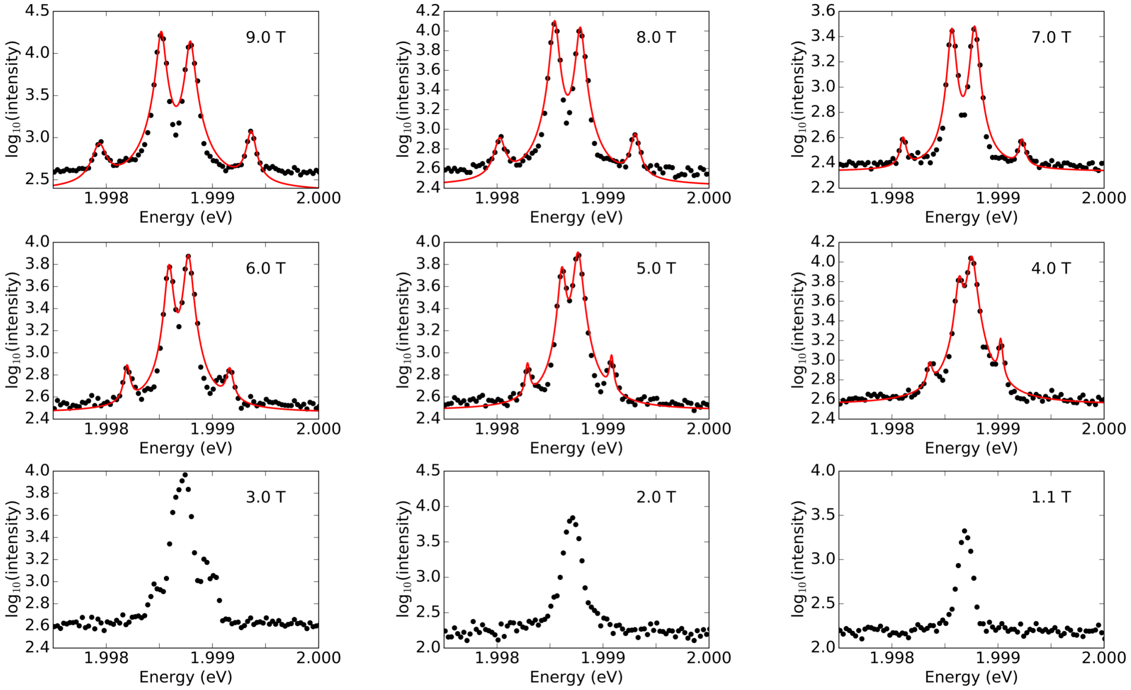


FIG. S5. Single monochromator spectra of D transitions at different magnetic fields at 1.7 K. Field at which data are acquired is indicated in the upper-right corner of each plot. Intensity (y-axis) on a $\log_{10}$ scale. Solid red lines are Lorentzian fits to the data. Unfitted spectra correspond to the omitted data points in the main text Fig. 5(e).

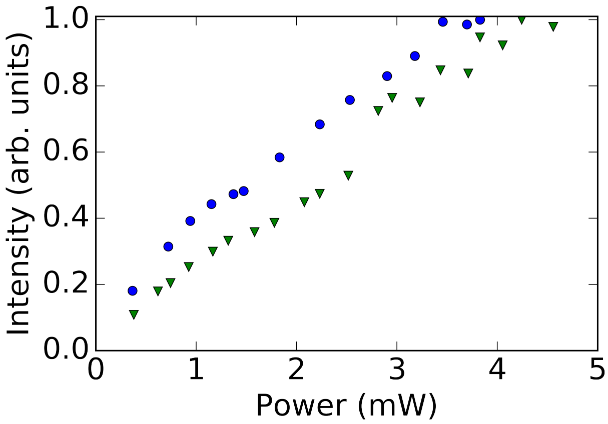


FIG. S6. Total emission intensity into the C and D zero-phonon lines as a function of incident power. The excitation power was not sufficient to get past the linear regime of the saturation curve.
